# Supplementary material for: What Color Scheme is More Effective in Assisting Readers to Locate Information in a Color-Coded Article?
Source: arXiv:2408.06494 source file (2024-08-26)
Supplement: Supplementary file 1 [file 7_appendix.tex]

\section{Annotation Prompt\label{app:prompt}}
Table \ref{table:zero-shot-table} shows the zero-shot prompt we used to annotate each segment in abstracts.
\begin{table*}
\centering
    \begin{tabular}{@{}p{\textwidth}@{}}
        \hline
        \textbf{Zero-shot Prompt} \\
        Classify the given text into one of the following labels.\\ \\

        [Background]: Text segments answer one or more of these questions: Why is this problem important?,
        What relevant works have been created before?, What is still missing in the previous works?, 
        What are the high-level research questions?, How might this help other research or researchers?\\
        
        [Purpose]: Text segments answer one or more of these questions: What specific things do the researchers want to do?, What specific knowledge do the researchers want to gain?, What specific hypothesis do the researchers want to test?\\
        
        [Method]: Text segments answer one or more of these questions: How did the researchers do the work or find what they sought?, What are the procedures and steps of the research?\\
        
        [Finding]: Text segments answer one or more of these questions: What did the researchers find out?, Did the proposed methods work?, Did the thing behave as the researchers expected?
        
        [Other]: Text fragments that do NOT fit into any of the four categories above. Text fragments that are NOT part of the article. Text fragments that are NOT in English. Text fragments that contains ONLY reference marks (e.g., "[1,2,3,4,5") or ONLY dates (e.g., "April 20, 2008"). Captions for figures and tables (e.g. "Figure 1: Experimental Result of ...", or "Table 1: The Typical Symptoms of ...") Formatting errors. I really don't know or I'm not sure.\\ \\
        
        FAQs\\
        
        1. This text fragment has terms that I don't understand. What should I do? Please use the context in the article to figure out the focus. You can look up terms you don't know if you feel like you need to understand them.\\
        2. This text fragment is too short to mean anything. What should I do? If the text fragment is too short to have significant meanings, you could consider the entire sentence and answer based on the entire sentence.\\
        3. This text fragment is NOT in English. What should I do? If the whole fragment (or the majority of words in the fragment) is in Non-English, please label it as "Other". If the majority of the words in this fragment are in English with a few non-English words, please judge the label normally.\\
        4. I'm not sure if this should be a "background" or a "finding." How do I tell? When a sentence occurs in the earlier part of an article, and it is presented as a known fact or looks authoritative, it is often a "background" information.\\
        5. Do "potential applications of the proposed work" count as "background" or "purpose"? It should be "background." The "purpose" refers to specific things the paper wants to achieve.\\
        6. If the article says it's a "literature review" (e.g., "We reviewed the literature" / "In this article, we review.." etc), would we classify those as finding/contribution or purpose? Most parts of a literature review paper should still be "background" or "purpose", and only the "insight" drew from a set of prior works can be viewed as a "finding/contribution".\\
        7. What should I do with the case study on a patient? Typically, it has a patient come in with a set of signs and symptoms in the ER, and then the patient gets assessed and diagnosed. The patient is admitted to the hospital ICU and tests are done and they may be diagnosed with something else. In such cases, please label the interventions done by the medical staff (e.g., CT scans, X-rays, and medications given) as "Method", and the patient's final result (e.g. the patient's pneumonia resolved and he was released from the hospital) as "Finding/Contribution".\\ \\
        
        Classify the following sentence into one of the label: Background, Purpose, Method, Finding, and Other. \\Provide answer in format of ```fragment-i []''' \\

        fragment-1 Text: ```\{\textbf{Sentence-1}\}'''\\
        Label: []\\

        fragment-2 Text: ```\{\textbf{Sentence-2}\}'''\\
        Label: []\\

        fragment-3 Text: ```\{\textbf{Sentence-3}\}'''\\
        Label: []\\
        ......\\
        \hline
    \end{tabular}
    \caption{Zero-shot prompt used when calling GPT-4~\cite{he2024chi}.}
    \label{table:zero-shot-table}
\end{table*}
